# Supplementary material for: Deep Reinforcement Learning for Vision-Based Robotic Grasping: A Simulated Comparative Evaluation of Off-Policy Methods
Source: arXiv:1802.10264 source file (2018-03-28)
Supplement: Supplementary file 1 [file appendix.tex]

\section{Appendix}

\subsection{Model}
\label{app:model}
 
In Figure~\ref{fig:critic_model} we show the model architecture we use for the Q-function.

\begin{figure}[h]
\begin{center}
\includegraphics[width=.3\textwidth]{images/network_arch_v2.eps}
\end{center}
\caption{
\label{fig:critic_model}
Architecture of Q-function for grasping.}
\end{figure}

\begin{figure}[h]
\begin{center}
\includegraphics[width=.3\textwidth]{images/network_arch_v2.eps}
\end{center}
\caption{
\label{fig:critic_model}
Architecture of Q-function for grasping.}
\end{figure}
